# Supplementary material for: "What Are You Trying to Do?" Semantic Typing of Event Processes
Source: arXiv:2010.06724 source file (2020-10-13)
Supplement: Supplementary file 1 [file 6Appendix.tex]

\clearpage
\appendix

\section{Appendices}
\label{sec:appendix}

.
